# Supplementary material for: Edge Reconstruction in a Quantum Spin Hall Insulator
Source: arXiv:2508.10726 source file (2026-07-11)
Supplement: Supplementary file 1 [file SuppMat.pdf]

# Supplemental Information: Edge Reconstruction in a Quantum Spin Hall Insulator

Rahul Soni,<sup>1,2</sup> Matthias Thamm,<sup>3</sup> Gonzalo Alvarez,<sup>4</sup> Bernd Rosenow,<sup>3</sup> and Adrian Del Maestro<sup>1,2,5</sup>

<sup>1</sup>*Department of Physics and Astronomy, University of Tennessee, Knoxville, Tennessee 37996, USA*

<sup>2</sup>*Institute for Advanced Materials and Manufacturing,  
University of Tennessee, Knoxville, Tennessee 37996, USA*

<sup>3</sup>*Institut für Theoretische Physik, Universität Leipzig, Brüderstrasse 16, 04103 Leipzig, Germany*

<sup>4</sup>*Computational Sciences and Engineering Division,  
Oak Ridge National Laboratory, Oak Ridge, TN 37831, USA*

<sup>5</sup>*Min H. Kao Department of Electrical Engineering and Computer Science,  
University of Tennessee, Knoxville, Tennessee 37996, USA*

(Dated: August 14, 2025)

## A. MEAN-FIELD APPROXIMATION

We employed a self-consistent mean-field approximation in real-space, based on the Hartree decoupling of the multi-orbital Hubbard interaction, retaining only the onsite intra- and inter-orbital density-density terms. The resulting mean-field interaction Hamiltonian is given by:

$$H_{\text{int}}^{\text{MF}} = U \sum_{\mathbf{r}, \alpha=s,p} [\langle n_{\mathbf{r},\alpha,\downarrow} \rangle n_{\mathbf{r},\alpha,\uparrow} + \langle n_{\mathbf{r},\alpha,\uparrow} \rangle n_{\mathbf{r},\alpha,\downarrow} - \langle n_{\mathbf{r},\alpha,\uparrow} \rangle \langle n_{\mathbf{r},\alpha,\downarrow} \rangle] + \left( U' - \frac{J_H}{2} \right) \sum_{\mathbf{r}} [\langle n_{\mathbf{r},s} \rangle n_{\mathbf{r},p} + \langle n_{\mathbf{r},p} \rangle n_{\mathbf{r},s} - \langle n_{\mathbf{r},s} \rangle \langle n_{\mathbf{r},p} \rangle], \quad (1)$$

where  $\langle n_{\mathbf{r},\alpha,\sigma} \rangle$  denotes the local charge order parameter for orbital  $\alpha$  and spin  $\sigma$  in unit cell  $\mathbf{r}$ . We solve for these order parameters self-consistently by minimizing the total mean-field energy at fixed chemical potential  $\mu = 0$ , corresponding to the grand-canonical ensemble. To ensure convergence, we initialize the iterative procedure with several random initial configurations (or seeds) and compare the energies of the different runs. To accelerate convergence, we employ Broyden mixing [1, 2], with a convergence threshold set to  $10^{-7}$ . All mean-field calculations are performed at low but finite temperature  $T = 0.0001$  (measured in units of the gap  $m$ ).

## Effect of helical-edge potential

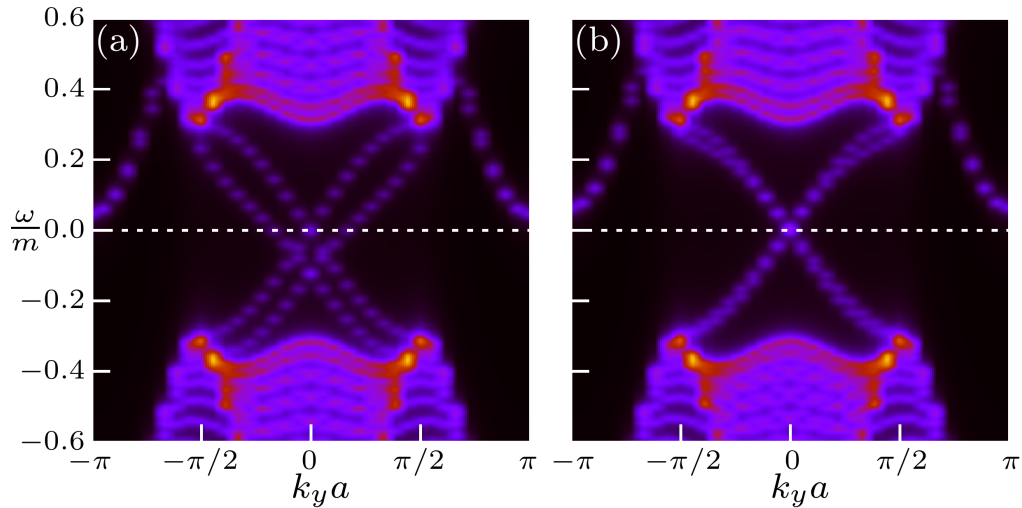

FIG. 1. Spectral function plots for different helical edge potentials at  $v_0 = 2.0$  for a  $36 \times 36$  system. Panels (a) shows the bands for  $\varepsilon_h = 0.0$  and (b) for  $\varepsilon_h = 0.3$ . The plot demonstrates the breakdown of mirror (left-right) symmetry between the left and right helical edges for  $\varepsilon_h = 0.0$ , that can be minimized with the consideration of an edge potential  $\varepsilon_h = 0.3$ .

We compute the single-particle spectral function in the mean field approximation on a cylinder (open along  $x$ , periodic along  $y$ ) with a smooth, spin-independent confining potential applied to one edge. For intermediate slopes the soft edge accumulates extra charge, producing a rigid shift of its Dirac cone (Fig. 1a). To make the two edges comparable, we include a localized repulsive edge term  $\varepsilon_h$ ; with  $\varepsilon_h = 0.3$  the Dirac points from the left and right helical edges coincide in mean field (Fig. 1b).

The same tendency appears in our many-body calculations using DMRG: with no additional edge term ( $\varepsilon_h = 0$ ), softening the confinement yields charge accumulation at the helical edge. Exploratory runs with a modest number of kept states indicate that the value  $\varepsilon_h = 0.4$  resembles the charge profile of a sharp, open-boundary helical edge.

## B. FINITE SIZE SCALING OF EXCHANGE COUPLING

To demonstrate that the exchange coupling  $J$  is not just a finite size effect, we perform finite size scaling from DMRG results using systems of sizes  $L_x \times 3$  with  $L_x \in \{12, 14, 16\}$ . We find that the coupling indeed increases with increasing system size  $L_x$  and a linear extrapolation to  $L_x \rightarrow \infty$  yields  $J_\infty \approx 0.0855$  (see Fig. 2).

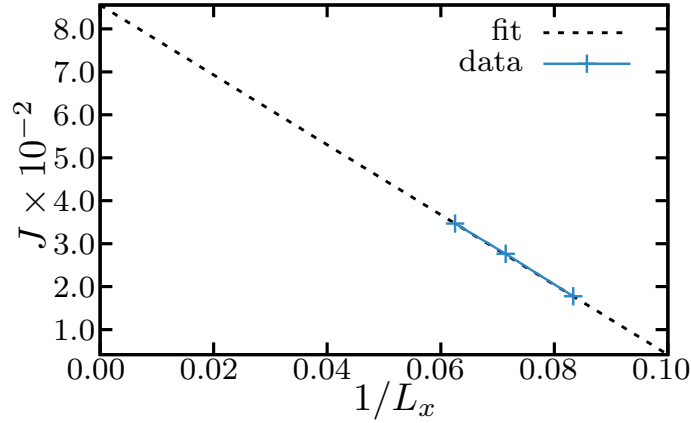

FIG. 2. Finite size scaling of the exchange coupling  $J$  as the function of  $1/L_x$ , obtained from our DMRG calculations of  $L_x \times 3$  cylinders. As the system grows the exchange become more robust.

## C. DOUBLY DEGENERATE GROUND STATE WAVEFUNCTION OF THREE SITE RING

As reported in the End Matter, we have performed exact diagonalization on a reduced Hamiltonian describing the physics of the interacting BHZ model on a three site ring to explore the structure of the low-lying reconstructed states. The associated wavefunctions corresponding to the doubly degenerate ground states with  $S_{\text{tot}}^z = \pm 1$  are given by  $|\Psi_{0,\pm 1}\rangle$ :

$$\begin{aligned}
 |\Psi_{0,-1}\rangle = & 0.573521 [-|\downarrow, \downarrow, 0\rangle_s + |\downarrow, 0, \downarrow\rangle_s - |0, \downarrow, \downarrow\rangle_s] |0, 0, 0\rangle_p \\
 & + 0.0526251 [|\downarrow, 0, 0\rangle_s |\downarrow, 0, 0\rangle_p + |0, \downarrow, 0\rangle_s |0, \downarrow, 0\rangle_p + |0, 0, \downarrow\rangle_s |0, 0, \downarrow\rangle_p] \\
 & - 0.0284747 [|\downarrow, 0, 0\rangle_s |0, \downarrow, 0\rangle_p + |\downarrow, 0, 0\rangle_s |0, 0, \downarrow\rangle_p + |0, \downarrow, 0\rangle_s |\downarrow, 0, 0\rangle_p + |0, \downarrow, 0\rangle_s |0, 0, \downarrow\rangle_p \\
 & + |0, 0, \downarrow\rangle_s |\downarrow, 0, 0\rangle_p + |0, 0, \downarrow\rangle_s |0, \downarrow, 0\rangle_p] + 0.00402652 |0, 0, 0\rangle_s [-|\downarrow, \downarrow, 0\rangle_p + |\downarrow, 0, \downarrow\rangle_p - |0, \downarrow, \downarrow\rangle_p] . \quad (2)
 \end{aligned}$$

The state  $|\Psi_{0,1}\rangle$  can be obtained from  $|\Psi_{0,-1}\rangle$  by swapping  $\downarrow \leftrightarrow \uparrow$ . The first excited state is:

$$\begin{aligned}
|\Psi_1\rangle = & 0.405946 \left[ |\uparrow, \downarrow, 0\rangle_s - |\uparrow, 0, \downarrow\rangle_s - |\downarrow, \uparrow, 0\rangle_s + |\uparrow, \uparrow, \downarrow\rangle_s + |\downarrow, 0, \uparrow\rangle_s - |\downarrow, \downarrow, \uparrow\rangle_s \right] |0, 0, 0\rangle_p \\
& - 0.0323504 \left[ |\uparrow, 0, 0\rangle_s |\downarrow, 0, 0\rangle_p + |0, \uparrow, 0\rangle_s |\downarrow, \downarrow, 0\rangle_p + |0, 0, \uparrow\rangle_s |0, 0, \downarrow\rangle_p \right] + 0.0201673 \\
& \left[ |\uparrow, 0, 0\rangle_s |0, \downarrow, 0\rangle_p + |\uparrow, 0, 0\rangle_s |0, 0, \downarrow\rangle_p + |0, \uparrow, 0\rangle_s |\downarrow, 0, 0\rangle_p + |0, \uparrow, 0\rangle_s |0, 0, \downarrow\rangle_p \right. \\
& \left. + |0, 0, \uparrow\rangle_s |\downarrow, 0, 0\rangle_p + |0, 0, \uparrow\rangle_s |0, \downarrow, 0\rangle_p \right] - 0.0201673 \left[ |0, \downarrow, 0\rangle_s |\uparrow, 0, 0\rangle_p + |0, 0, \downarrow\rangle_s |\uparrow, 0, 0\rangle_p \right. \\
& \left. + |\downarrow, 0, 0\rangle_s |0, \uparrow, 0\rangle_p + |0, 0, \downarrow\rangle_s |0, \uparrow, 0\rangle_p + |\downarrow, 0, 0\rangle_s |0, 0, \uparrow\rangle_p + |0, \downarrow, 0\rangle_s |0, 0, \uparrow\rangle_p \right] \\
& + 0.00260901 |0, 0, 0\rangle_s \left[ |\uparrow, \downarrow, 0\rangle_p - |\uparrow, 0, \downarrow\rangle_p - |\downarrow, \uparrow, 0\rangle_p + |0, \uparrow, \downarrow\rangle_p + |\downarrow, 0, \uparrow\rangle_p - |0, \downarrow, \uparrow\rangle_p \right] . \tag{3}
\end{aligned}$$

- 
- [1] C. G. Broyden, [Mathematics of Computation](#) **19**, 577 (1965).  
[2] A. Baran, A. Bulgac, M. M. Forbes, G. Hagen, W. Nazarewicz, N. Schunck, and M. V. Stoitsov, [Phys. Rev. C](#) **78**, 014318 (2008).
